# Supplementary material for: Born-Oppenheimer Dynamics, Electronic Friction, and the Inclusion of Electron-Electron Interactions
Source: arXiv:1703.04717 ancillary file (2017-06-29)
Supplement: Supplementary file 1 [file SupportingInfo18.pdf]

# Born-Oppenheimer Dynamics, Electronic Friction, and the Inclusion of Electron-Electron Interactions (Supplemental Material)

Wenjie Dou,[1] Gaohan Miao,[1] and Joseph E. Subotnik[1,2]
[1]*Department of Chemistry, University of Pennsylvania, Philadelphia, Pennsylvania 19104, USA*
[2]*Stanford PULSE Institute, SLAC National Accelerator Laboratory, Menlo Park, California 94025, USA*

## I. DERIVING THE ELECTRONIC FRICTION TENSOR AND RANDOM FORCE

In this Supplemental Material (SM), we begin by deriving the electronic friction (Eq. 7) and random force (Eq. 9) associated with Born-Oppenheimer (BO) motion. This will be done in two ways.

### A. A Heuristic, Almost Correct Derivation

For our first approach, we provide a heuristic, almost correct derivation of BO Langevin dynamics. We assume semiclassical dynamics, where the equation of motion for the nuclear trajectories ($R_\alpha$, $P_\alpha$) and the electronic density matrix ($\hat{\rho}$) are given by Newton's equations and the von Neumann equation respectively,

$$-m_\alpha \ddot{R}_\alpha = \partial_\alpha \hat{H} \tag{15}$$

$$\dot{\hat{\rho}} = -\hat{\hat{\mathcal{L}}}\hat{\rho} \tag{16}$$

$\alpha$ (or $\nu$) indexes nuclear degrees of freedom (DoF's). $\hat{\hat{\mathcal{L}}}$ is the Liouvillian superoperator. The Liouville operator is standard, $-\hat{\hat{\mathcal{L}}}(\cdot) = -\frac{i}{\hbar}[\hat{H}, \cdot]$. The electronic density matrix $\hat{\rho}$ satisfies $tr_e(\hat{\rho}) = 1$, where $tr_e$ implies tracing over all electronic DoF's.

To derive Langevin dynamics, we first rewrite Eq. 15 as

$$-m_\alpha \ddot{R}_\alpha = tr_e(\partial_\alpha \hat{H}\hat{\rho}) + (\partial_\alpha \hat{H} - tr_e(\partial_\alpha \hat{H}\hat{\rho})) \tag{17}$$

where we have divided the total force into the average force and a random force.

We proceed to consider the electronic dynamics (Eq. 16). If the nuclei do not move, we assume there is a large number of electronic DoF's possible, so that the electrons will reach a steady state $\hat{\rho} = \hat{\rho}_{ss}$, where $-\hat{\hat{\mathcal{L}}}\hat{\rho}_{ss} = 0$.

Now if the nuclear motion is considered and nucleus $\nu$ moves by $\dot{R}_\nu dt$ over time step $dt$, we define

$$\hat{\rho} = \hat{\rho}_{ss} + \Delta\hat{\rho} \tag{18}$$

If we plug the above equation into Eq. 16 and use the definition of the steady state solution, we find

$$\dot{\hat{\rho}} = -\hat{\hat{\mathcal{L}}}\Delta\hat{\rho} \tag{19}$$

We now invoke the key, adiabatic approximation. In the adiabatic limit, the electrons reach a steady state on a timescale much faster than the typical timescale of nuclear motion, such that the difference between $\hat{\rho}$ and $\hat{\rho}_{ss}$ (which is $\Delta\hat{\rho}$) is very small. Hence, we approximate $\hat{\rho}$ by $\hat{\rho}_{ss}$ in Eq. 19 and formally invert the Liouvillian,

$$\Delta\hat{\rho} \approx -\hat{\hat{\mathcal{L}}}^{-1}\dot{\hat{\rho}}_{ss} = -\sum_\nu \dot{R}_\nu \hat{\hat{\mathcal{L}}}^{-1}\partial_\nu \hat{\rho}_{ss} \tag{20}$$

Then, if we plug Eqs. 18 and 20 back into Eq. 17, we arrive at a closed Langevin equation for the nuclei,

$$-m_\alpha \ddot{R}_\alpha = -F_\alpha + \sum_\nu \gamma_{\alpha\nu}\dot{R}_\nu - \delta\hat{F}_\alpha \tag{21}$$

Here,

$$F_\alpha = -tr_e\big(\partial_\alpha \hat{H}\hat{\rho}_{ss}\big) \tag{22}$$

$$\gamma_{\alpha\nu} = -tr_e\Big(\partial_\alpha \hat{H}\hat{\hat{\mathcal{L}}}^{-1}\partial_\nu \hat{\rho}_{ss}\Big) \tag{23}$$

$$\delta\hat{F}_\alpha = -\partial_\alpha \hat{H} + tr_e(\partial_\alpha \hat{H}\hat{\rho}_{ss}) \tag{24}$$

In Eq. 24, when evaluating the random force, we have replaced $\hat{\rho}$ by $\hat{\rho}_{ss}$, which is consistent with our adiabatic approximation.

We now look closely at the friction (Eq. 23). Using the identify $\hat{\hat{\mathcal{L}}}^{-1} = \lim_{\eta\to 0^+}\int_0^\infty dt e^{-\left(\hat{\hat{\mathcal{L}}}+\eta\right)t}$, we can rewrite $\gamma_{\alpha\nu}$ as the integral of a correlation function,

$$\gamma_{\alpha\nu} = -\lim_{\eta\to 0^+}\int_0^\infty dt\, tr_e\Big(\partial_\alpha \hat{H} e^{-\left(\hat{\hat{\mathcal{L}}}+\eta\right)t}\partial_\nu \hat{\rho}_{ss}\Big) \tag{25}$$

where $e^{-\hat{\hat{\mathcal{L}}}t}(\cdot) = e^{-i\hat{H}t/\hbar}(\cdot)e^{i\hat{H}t/\hbar}$ is the Liouvillian propagator. The above equation can be recast into the energy domain,

$$\begin{aligned}
\gamma_{\alpha\nu} &= -\lim_{\eta\to 0^+}\int_0^\infty dt\, tr_e\Big(\partial_\alpha \hat{H} e^{-i(\hat{H}-i\eta)t/\hbar}\partial_\nu \hat{\rho}_{ss} e^{i(\hat{H}+i\eta)t/\hbar}\Big)\\
&= -\lim_{\eta\to 0^+}\int_0^\infty dt\int_0^\infty dt'\, tr_e\Big(\partial_\alpha \hat{H} e^{-i(\hat{H}-i\eta)t/\hbar}\partial_\nu \hat{\rho}_{ss} e^{i(\hat{H}+i\eta)t'/\hbar}\Big)\delta(t-t')\\
&= -\lim_{\eta\to 0^+}\int_{-\infty}^\infty \frac{d\epsilon}{2\pi\hbar}\int_0^\infty dt\int_0^\infty dt'\, tr_e\Big(\partial_\alpha \hat{H} e^{-i(\hat{H}-i\eta)t/\hbar}\partial_\nu \hat{\rho}_{ss} e^{i(\hat{H}+i\eta)t'/\hbar}\Big)e^{i\epsilon(t-t')/\hbar}\\
&= -\lim_{\eta\to 0^+}\hbar\int_{-\infty}^\infty \frac{d\epsilon}{2\pi}\, tr_e\Big(\partial_\alpha \hat{H}\frac{1}{\epsilon-\hat{H}+i\eta}\partial_\nu \hat{\rho}_{ss}\frac{1}{\epsilon-\hat{H}-i\eta}\Big)
\end{aligned} \tag{26}$$

Note that this friction tensor agrees exactly with Eq. 8 in the body of the letter.

Next, consider the random force $\delta\hat{F}_\alpha$ and the corresponding correlation function:

$$D_{\alpha\nu}(t) = tr_e(e^{i\hat{H}t/\hbar}\delta\hat{F}_\alpha e^{-i\hat{H}t/\hbar}\delta\hat{F}_\nu\hat{\rho}_{ss}) \tag{27}$$

In the Markovian limit, we assume that, as far as time-dependence is concerned, $D_{\alpha\nu}(t)$ is simply a delta function at time zero:

$$D_{\alpha\nu}(t) \to 2\bar{D}_{\alpha\nu}\delta(t) \tag{28}$$

The assumption of a Markovian corrrelation function is consistent with adiabatic dynamicis (i.e. fast electronic motion). Taking the integral for $t$ from 0 to $\infty$, we find:

$$\bar{D}_{\alpha\nu} = \int_0^\infty dt\, tr_e(e^{i\hat{H}t/\hbar}\delta\hat{F}_\alpha e^{-i\hat{H}t/\hbar}\delta\hat{F}_\nu\hat{\rho}_{ss}) \tag{29}$$

Of course, in a realistic simulation, the random force $\delta\hat{F}_\alpha$ is replaced by a random number $\zeta_\alpha$, which satisfies

$$\langle\zeta_\alpha(t)\rangle = 0,\ \langle\zeta_\alpha(t)\zeta_\nu(t')\rangle = \bar{D}_{\alpha\nu}\delta(t-t') \tag{30}$$

Here, we note that $\bar{D}_{\alpha\nu}$ is not guaranteed to be real or symmetric and does not agree exactly with Eq. 9 in the body of the letter. To recover the correct, real and symmetric, random force, we will now start from the quantum classical Liouville equation (QCLE).

### B. Derivation of Fokker-Planck equation from the QCLE

For our second approach, and to derive the proper electronic friction tensor and go beyond the heuristic derivation above, in a spirit similar to Ref. [1], we start our derivation from the quantum-classical Liouville equation (QCLE) [2],

$$\partial_t\hat{\mathcal{W}}(\mathbf{R},\mathbf{P},t) = \{\hat{H}_{tot},\hat{\mathcal{W}}\}_a - \hat{\hat{\mathcal{L}}}\hat{\mathcal{W}} \tag{31}$$

Here $\hat{\mathcal{W}}$ is the density matrix in phase space $(\mathbf{R},\mathbf{P})$. $\{\cdot,\cdot\}_a$ is the anti-symmetrized Poisson bracket $\{\cdot,\cdot\}$,

$$\{\hat{H}_{tot},\hat{\mathcal{W}}\}_a = \frac{1}{2}\{\hat{H}_{tot},\hat{\mathcal{W}}\} - \frac{1}{2}\{\hat{\mathcal{W}},\hat{H}_{tot}\} \tag{32}$$

As before, we will assume that the kinetic and potential energies are separable within the total Hamiltonian,

$$\hat{H}_{tot}(\mathbf{R},\mathbf{P}) = \hat{H}(\mathbf{R}) + \sum_\alpha \frac{P_\alpha^2}{2m_\alpha} \tag{33}$$

such that,

$$\{\hat{H}_{tot},\hat{\mathcal{O}}\}_a = -\sum_\alpha \frac{P_\alpha}{m_\alpha}\partial_\alpha\hat{\mathcal{O}} + \frac{1}{2}\sum_\alpha(\partial_\alpha\hat{H}\frac{\partial\hat{\mathcal{O}}}{\partial P_\alpha} + \frac{\partial\hat{\mathcal{O}}}{\partial P_\alpha}\partial_\alpha\hat{H}) \tag{34}$$

Since we assume there is always a manifold of electronic DoF's, the Liouvillian $\hat{\hat{\mathcal{L}}}$ admits a local steady state solution $\hat{\rho}_{ss}$,

$$\hat{\hat{\mathcal{L}}}(\mathbf{R})\hat{\rho}_{ss}(\mathbf{R}) = 0. \tag{35}$$

$\hat{\rho}_{ss}$ is normalized, $tr_e(\hat{\rho}_{ss}) = 1$. We will further define

$$\hat{\mathcal{W}}(\mathbf{R},\mathbf{P},t) = \mathcal{A}(\mathbf{R},\mathbf{P},t)\hat{\rho}_{ss}(\mathbf{R}) + \hat{\mathcal{B}}(\mathbf{R},\mathbf{P},t) \tag{36}$$

where $\mathcal{A}$ is the probability density in phase space, $\mathcal{A} = tr_e(\hat{\mathcal{W}})$. In the adiabatic limit, $\hat{\mathcal{B}}$ should be very small compared to $\mathcal{A}\hat{\rho}_{ss}$, and at steady state, we expect $\hat{\mathcal{B}} = 0$.

Using Eq. 31, we can write an equation of motion (EOM) for $\mathcal{A}$

$$\partial_t\mathcal{A} = -\sum_\alpha \frac{P_\alpha}{m_\alpha}\partial_\alpha\mathcal{A} + \sum_\alpha tr_e(\partial_\alpha\hat{H}\hat{\rho}_{ss})\frac{\partial\mathcal{A}}{\partial P_\alpha} + \sum_\alpha tr_e(\partial_\alpha\hat{H}\frac{\partial\hat{\mathcal{B}}}{\partial P_\alpha}) \tag{37}$$

and for $\hat{\mathcal{B}}$,

$$\partial_t\hat{\mathcal{B}} = \{\hat{H}_{tot},\hat{\mathcal{B}}\}_a - \hat{\rho}_{ss}tr_e\{\hat{H}_{tot},\hat{\mathcal{B}}\}_a + \{\hat{H}_{tot},\mathcal{A}\hat{\rho}_{ss}\}_a - \hat{\rho}_{ss}tr_e\{\hat{H}_{tot},\mathcal{A}\hat{\rho}_{ss}\}_a - \hat{\hat{\mathcal{L}}}\hat{\mathcal{B}} \tag{38}$$

In the adiabatic limit, the nuclear motion is much slower than electronic transition. Just as in Ref. [1], we can approximate Eq. 38 as

$$\hat{\hat{\mathcal{L}}}\hat{\mathcal{B}} = \{\hat{H}_{tot},\mathcal{A}\hat{\rho}_{ss}\}_a - \hat{\rho}_{ss}tr_e\{\hat{H}_{tot},\mathcal{A}\hat{\rho}_{ss}\}_a \tag{39}$$

Inverting the Liouvillian in the above equation, and plugging the solution for $\hat{\mathcal{B}}$ back to Eq. 37, we arrive at a closed Fokker-Planck equation for the probability density $\mathcal{A}$,

$$\partial_t\mathcal{A} = -\sum_\alpha \frac{P_\alpha}{m_\alpha}\partial_\alpha\mathcal{A} - \sum_\alpha F_\alpha\frac{\partial\mathcal{A}}{\partial P_\alpha} + \sum_{\alpha\nu}\gamma_{\alpha\nu}\frac{\partial}{\partial P_\alpha}(\frac{P_\nu}{m_\nu}\mathcal{A}) + \sum_{\alpha\nu}\bar{D}^S_{\alpha\nu}\frac{\partial^2\mathcal{A}}{\partial P_\alpha\partial P_\nu} \tag{40}$$

Here, the mean force $F_\alpha$ and friction $\gamma_{\alpha\nu}$ have the same forms as given by Eq. 22 and Eq. 23. However, the correlation function of the random force in Eq. 40 is given by

$$\bar{D}^S_{\alpha\nu} = \frac{1}{2}tr_e\Big(\partial_\alpha\hat{H}\hat{\hat{\mathcal{L}}}^{-1}(\partial_\nu\hat{H}\hat{\rho}_{ss} + \hat{\rho}_{ss}\partial_\nu\hat{H} - 2\hat{\rho}_{ss}tr_e(\hat{\rho}_{ss}\partial_\nu\hat{H}))\Big) \tag{41}$$

The above equation can be rewritten in terms of time correlation functions,

$$\bar{D}^S_{\alpha\nu} = \frac{1}{2}\int_0^\infty dt\, tr_e\big(e^{i\hat{H}t/\hbar}\delta\hat{F}_\alpha e^{-i\hat{H}t/\hbar}(\delta\hat{F}_\nu\hat{\rho}_{ss} + \hat{\rho}_{ss}\delta\hat{F}_\nu)\big) = \mathrm{Re}\left(\bar{D}_{\alpha\nu}\right) \tag{42}$$

proving that $\bar{D}^S_{\alpha\nu}$ is always real. Also, it is easy to show that $\bar{D}^S_{\alpha\nu}$ is also symmetric along $\alpha$ and $\nu$ for real-valued $\hat{H}$ and $\hat{\rho}_{ss}$, i.e. $\bar{D}^S_{\nu\alpha} = \bar{D}^S_{\alpha\nu}$.

In Sec. VII of this SM, we show the non-Markovian version of this Fokker-Planck equation.

## II. THE SECOND FLUCTUATION-DISSIPATION THEOREM

To prove the second fluctuation-dissipation theorem (Eq. 11 in the body of the letter), we will use the eigenvalue or Lehmann representation of the electronic manifold, $\hat{H}|a\rangle = E_a|a\rangle$:

$$\begin{aligned}\gamma_{\alpha\nu} &= -\sum_{ab}\int_0^\infty dt\,\langle a|\partial_\alpha\hat{H}|b\rangle e^{-iE_bt/\hbar}\langle b|\partial_\nu\hat{\rho}_{ss}|a\rangle e^{iE_at/\hbar}\\ &= -\hbar\sum_{ab}\langle a|\partial_\alpha\hat{H}|b\rangle\langle b|\partial_\nu\hat{\rho}_{ss}|a\rangle\frac{i}{E_b-E_a+i\eta}\end{aligned} \tag{43}$$

Here, $\eta$ is an infinitesimially small positive number and we restrict ourselves to real-valued $\hat{H}$ and $\hat{\rho}_{ss}$. Since $\gamma_{\alpha\nu}$ is real, we can take the real part of the above equation

$$\gamma_{\alpha\nu} = -\pi\hbar\sum_{ab}\langle a|\partial_\alpha\hat{H}|b\rangle\langle b|\partial_\nu\hat{\rho}_{ss}|a\rangle\delta(E_b-E_a) \tag{44}$$

At equilibrium, $\hat{\rho}_{ss} = \frac{1}{Z}e^{-\beta\hat{H}}$. Let us denote $\rho_a = \frac{1}{Z}e^{-\beta E_a}$. The following identities can be used,

$$\partial_\nu\langle b|\hat{\rho}_{ss}|a\rangle = \delta_{ab}\partial_\nu\rho_a = \langle b|\partial_\nu\hat{\rho}_{ss}|a\rangle + \frac{e^{-\beta E_b}-e^{-\beta E_a}}{Z}\langle b|\partial_\nu|a\rangle \tag{45}$$

$$\partial_\nu\langle b|\hat{H}|a\rangle = \delta_{ab}\partial_\nu E_a = \langle b|\partial_\nu\hat{H}|a\rangle + (E_b-E_a)\langle b|\partial_\nu|a\rangle \tag{46}$$

such that can rewrite $\langle b|\partial_\nu\hat{\rho}_{ss}|a\rangle$ as follows:

$$\begin{aligned}\langle b|\partial_\nu\hat{\rho}_{ss}|a\rangle &= \delta_{ab}\partial_\nu\rho_a - \frac{1}{Z}\frac{e^{-\beta E_b}-e^{-\beta E_a}}{E_b-E_a}(\delta_{ab}\partial_\nu E_a - \langle b|\partial_\nu\hat{H}|a\rangle)\\ &= -\delta_{ab}\frac{1}{Z}\rho_a\partial_\nu Z + \frac{1}{Z}\frac{e^{-\beta E_b}-e^{-\beta E_a}}{E_b-E_a}\langle b|\partial_\nu\hat{H}|a\rangle\\ &= \beta\, tr_e(\partial_\nu\hat{H}\hat{\rho}_{ss})\langle b|\hat{\rho}_{ss}|a\rangle + \frac{1}{Z}\frac{e^{-\beta E_b}-e^{-\beta E_a}}{E_b-E_a}\langle b|\partial_\nu\hat{H}|a\rangle\end{aligned} \tag{47}$$

Above, we have used the fact that $\delta_{ab}\frac{e^{-\beta E_b}-e^{-\beta E_a}}{E_b-E_a} = \delta_{ab}\partial_{E_a}e^{-\beta E_a} = -\beta\delta_{ab}e^{-\beta E_a}$.

The second term in Eq. 47 gives a force-force correlation function:

$$\begin{aligned}&-\pi\hbar\sum_{ab}\langle a|\partial_\alpha\hat{H}|b\rangle\langle b|\partial_\nu\hat{H}|a\rangle\frac{1}{Z}\frac{e^{-\beta E_b}-e^{-\beta E_a}}{E_b-E_a}\delta(E_b-E_a)\\ &= \beta\pi\hbar\sum_{ab}\langle a|\partial_\alpha\hat{H}|b\rangle\langle b|\partial_\nu\hat{H}|a\rangle\frac{e^{-\beta E_b}}{Z}\delta(E_b-E_a)\\ &= \frac{\beta\pi\hbar}{2}\sum_{ab}\langle a|\partial_\alpha\hat{H}|b\rangle\langle b|\partial_\nu\hat{H}|a\rangle\frac{e^{-\beta E_b}+e^{-\beta E_a}}{Z}\delta(E_b-E_a)\\ &= \frac{\beta\pi\hbar}{2}\sum_{ab}\langle a|\partial_\alpha\hat{H}|b\rangle\langle b|\partial_\nu\hat{H}\hat{\rho}_{ss}+\hat{\rho}_{ss}\partial_\nu\hat{H}|a\rangle\delta(E_b-E_a)\\ &= \frac{\beta}{2}\int_0^\infty dt\, tr_e(\partial_\alpha\hat{H}e^{-i\hat{H}t/\hbar}(\partial_\nu\hat{H}\hat{\rho}_{ss}+\hat{\rho}_{ss}\partial_\nu\hat{H})e^{i\hat{H}t/\hbar})\end{aligned} \tag{48}$$

The first term in Eq. 47 gives a mean-field contriibution to the friction:

$$\begin{aligned}&-\pi\hbar\beta\sum_{ab}\langle a|\partial_\alpha\hat{H}|b\rangle\langle b|tr_e(\partial_\nu\hat{H}\hat{\rho}_{ss})\hat{\rho}_{ss}|a\rangle\delta(E_b-E_a)\\ &= -\beta\int_0^\infty dt\, tr_e(\partial_\alpha\hat{H}e^{-i\hat{H}t/\hbar}tr_e(\partial_\nu\hat{H}\hat{\rho}_{ss})\hat{\rho}_{ss}e^{i\hat{H}t/\hbar})\end{aligned} \tag{49}$$

Finally, summing up the two contributions, we find that the final friction can be rewritten in terms of a correlation function of the random force $\delta\hat{F}$ in Eq. 24:

$$\begin{aligned}\gamma_{\alpha\nu} &= -\frac{\beta}{2}\int_0^\infty dt\, tr_e(\partial_\alpha \hat{H} e^{-i\hat{H}t/\hbar}(\delta\hat{F}_\nu\hat{\rho}_{ss} + \hat{\rho}_{ss}\delta\hat{F}_\nu)e^{i\hat{H}t/\hbar}) \\ &= \frac{\beta}{2}\int_0^\infty dt\, tr_e(\delta\hat{F}_\alpha e^{-i\hat{H}t/\hbar}(\delta\hat{F}_\nu\hat{\rho}_{ss} + \hat{\rho}_{ss}\delta\hat{F}_\nu)e^{i\hat{H}t/\hbar}) = \beta\bar{D}^S_{\alpha\nu}\end{aligned} \tag{50}$$

Thus, the second fluctuation-dissipation theorem has been proven.

## III. DETAILS OF NRG CALCULATION

To calculate the friction at equilibrium, we rewrite Eq. 50 in the eigenvalue or Lehmann representation:

$$\gamma_{\alpha\nu} = \frac{\pi\hbar\beta}{2}\sum_{ab}\langle a|\delta\hat{F}_\alpha|b\rangle\langle b|\delta\hat{F}_\nu|a\rangle\frac{e^{-\beta E_b}+e^{-\beta E_a}}{Z}\delta(E_b - E_a) \tag{51}$$

Now, in an numerical renormalization group (NRG) calculation, the electronic continuum is mapped onto a semi-infinite chain, with coupling between the nearest sites exponentially decaying. The typical energy scale for the Nth site on the chain is

$$\omega_N = \frac{1}{2}(1+\Lambda^{-1})\Lambda^{-(N-1)/2} \tag{52}$$

$\Lambda$ is the logarithmic discretization parameter. For a given temperature, the semi-infinite chain is truncated at that site $N$ where $\omega_N$ is on the order of T, i.e.

$$N = \left[1 - 2\frac{\log(2k_BT/(1+\Lambda^{-1}))}{\log(\Lambda)}\right] \tag{53}$$

In the above equation, the squared bracket signifies the floor function, such that $N$ is always an integer.

Thus, to calculate friction with NRG, one iteratively diagonalizes the semi-infinite chain up to the Nth site and the resulting eigenstates and eigenvalues are plugged into Eq. 51. For a practical calculation, the delta function in Eq. 51 is chosen to be a gaussian with a width $\eta_N$.

$$\delta(E_b - E_a) = \frac{1}{\eta_N\sqrt{\pi}}e^{-\frac{(E_b-E_a)^2}{\eta_N^2}} \tag{54}$$

As is common with NRG calculations, $\eta_N$ is chosen to be $0.3\omega_N - 0.8\omega_N$ [3].

In our calculations, 500 states are kept for each iteration. The logarithmic discretization parameter is $\Lambda = 2$, and $\eta_N = 0.8\omega_N$.

## IV. MEAN-FIELD THEORY FRICTION

In Fig. 1 of the letter, we plotted the electronic friction according to mean-field theory (MFT) for the Anderson-Holstein model. We now show how such electronic friction is calculated. The basic premise is that we construct a one-electron mean-field Hamiltonian:

$$\hat{H}_{MF} = E_{eff}\sum_\sigma \hat{d}^+_\sigma\hat{d}_\sigma + \sum_{k\sigma}V_k(\hat{d}^+_\sigma\hat{c}_{k\sigma} + \hat{c}^+_{k\sigma}\hat{d}_\sigma) + \sum_{k\sigma}\epsilon_k\hat{c}^+_{k\sigma}\hat{c}_{k\sigma} - Un_\uparrow n_\downarrow \tag{55}$$

We assume, because there is no external field to break spin-symmetry, that $n_\uparrow = n_\downarrow$, where $n_\sigma \equiv \left\langle \hat{d}^+_\sigma\hat{d}_\sigma\right\rangle$. Furthermore, $E_{eff}$ is given by

$$E_{eff} = E(x) + n_\uparrow U \tag{56}$$

and

$$n_{\uparrow} = \int \frac{d\epsilon}{2\pi} \frac{\Gamma}{(\epsilon - E_{eff})^2 + (\Gamma/2)^2} f(\epsilon) \tag{57}$$

Eq. 56 and Eq. 57 have to be solved self-consistently. The final electronic friction is given by [4]

$$\gamma = -2 \times \frac{\hbar}{2} (\partial_x E_{eff})^2 \int \frac{d\epsilon}{2\pi} \left( \frac{\Gamma}{(\epsilon - E_{eff})^2 + (\Gamma/2)^2} \right)^2 \partial_\epsilon f(\epsilon) \tag{58}$$

The factor 2 in the above equation counts for spin degeneracy.

## V. QUADRATIC HAMILTONIAN

We now show our results (mean force, friction and correlation of random force) for the case of a quadratic electronic Hamiltonian. Our goal is to show that the friction and random force presented in the main body of the letter are in complete agreement with Head-Gordon and Tully [5].

To begin our derivation, as usual, the total Hamiltonian $\hat{H}_{tot}$ is separated into the electronic Hamiltonian $\hat{H}$ and nuclear kinetic Hamiltonian,

$$\hat{H}_{tot} = \hat{H} + \sum_{\alpha} \frac{P_\alpha^2}{2m^\alpha} \tag{59}$$

The electronic Hamiltonian is written with the following notation:

$$\hat{H} = \sum_{pq} h_{qp}(\mathbf{R}) \hat{d}_p^+ \hat{d}_q + U_0(\mathbf{R}) \tag{60}$$

$U_0(\mathbf{R})$ represents the component of the potential energy for the nuclei that is uncoupled from the electronic orbitals ($p$, $q$). We remind the reader that the Hamiltonian in Eq. 60 is exactly the same as (or even slighlty more general than) the Hamiltonian used by von Oppen *et al* in Ref. [6]. In Ref. [6], the electronic Hamiltonian is divided into dot, metal and coupling, which are all quadratic. That being said, we have rewritten this quadratic Hamiltonian in a compact way, without specifying dot, metal and coupling Hamiltonian, such that the matrix elements $h_{pq}(\mathbf{R})$ represent (inclusively) the dot energy, the coupling between dots, the coupling between dots and metal, the energy levels of the metal nearby, etc. Of course, $h_{pq}(\mathbf{R})$ is a very general notation, and specific matrix elements may or may not depend on the nuclear DoFs ($\mathbf{R}$).

### A. Mean Force

The mean force is easy to evaluate (using Eq. 22),

$$F_\alpha \ = \ -tr_e\big(\partial_\alpha \hat{H} \hat{\rho}_{ss}\big) = -\partial_\alpha U_0(\mathbf{R}) - \sum_{pq} \partial_\alpha h_{qp}(\mathbf{R}) tr_e(\hat{d}_p^+ \hat{d}_q \hat{\rho}_{ss}) \tag{61}$$

If we define $\sigma_{pq}^{ss} = tr_e(\hat{d}_p^+ \hat{d}_q \hat{\rho}_{ss})$, the mean force can be written as

$$F_\alpha \ = \ = -\partial_\alpha U_0 - \mathrm{Tr}_m(\partial_\alpha \underline{\underline{h}}\, \underline{\underline{\sigma}}^{ss}) \tag{62}$$

Here $\mathrm{Tr}_m$ implies summing over electronic orbitals, such that

$$\mathrm{Tr}_m(\partial_\alpha \underline{\underline{h}}\, \underline{\underline{\sigma}}^{ss}) = \sum_{pq} \partial_\alpha h_{qp} \sigma_{pq}^{ss}. \tag{63}$$

### B. Electronic Friction

We now evaluate the friction using Eq. 25:

$$\gamma_{\alpha\nu} = -\int_0^\infty dt\, tr_e\left(\partial_\alpha \hat{H} e^{-i\hat{H}t/\hbar}\partial_\nu\hat{\rho}_{ss}e^{i\hat{H}t/\hbar}\right) \tag{64}$$

Note that $U_0(\mathbf{R})$ does not contribute to the friction, because

$$tr_e\left(\partial_\alpha U_0 e^{-i\hat{H}t/\hbar}\partial_\nu\hat{\rho}_{ss}e^{i\hat{H}t/\hbar}\right) = \partial_\alpha U_0\, tr_e\left(\partial_\nu\hat{\rho}_{ss}\right) = 0. \tag{65}$$

Here, we have used the fact that $tr_e\left(\hat{\rho}_{ss}\right) = 1$. The friction can be rewritten as

$$\begin{aligned}\gamma_{\alpha\nu} &= -\int_0^\infty dt\, tr_e\left(e^{i\hat{H}t/\hbar}\partial_\alpha\hat{H}e^{-i\hat{H}t/\hbar}\partial_\nu\hat{\rho}_{ss}\right)\\ &= -\int_0^\infty dt\,\sum_{mn}\partial_\alpha h_{nm} tr_e\left(e^{i\hat{H}t/\hbar}\hat{d}_m^+\hat{d}_n e^{-i\hat{H}t/\hbar}\partial_\nu\hat{\rho}_{ss}\right)\end{aligned} \tag{66}$$

We proceed to evaluate

$$\hat{d}_m^+(t) = e^{i\hat{H}t/\hbar}\hat{d}_m^+e^{-i\hat{H}t/\hbar} \tag{67}$$

$$\hat{d}_n(t) = e^{i\hat{H}t/\hbar}\hat{d}_n e^{-i\hat{H}t/\hbar} \tag{68}$$

The time derivatives of these operators are

$$\dot{\hat{d}}_m^+(t) = e^{i\hat{H}t}\frac{i}{\hbar}[\hat{H},\hat{d}_m^+]e^{-i\hat{H}t} = \frac{i}{\hbar}\sum_a h_{ma}\hat{d}_a^+(t) \tag{69}$$

$$\dot{\hat{d}}_n(t) = e^{i\hat{H}t}\frac{i}{\hbar}[\hat{H},\hat{d}_n]e^{-i\hat{H}t} = -\frac{i}{\hbar}\sum_b h_{bn}\hat{d}_b(t) \tag{70}$$

The above equations can be solved

$$e^{i\hat{H}t}\hat{d}_m^+e^{-i\hat{H}t/\hbar} = \sum_a (e^{i\underline{\underline{h}}t/\hbar})_{ma}\hat{d}_a^+ \tag{71}$$

$$e^{i\hat{H}t}\hat{d}_n e^{-i\hat{H}t/\hbar} = \sum_b (e^{-i\underline{\underline{h}}t/\hbar})_{bn}\hat{d}_b \tag{72}$$

If we plug the above equations into Eq. 66, we find:

$$\begin{aligned}\gamma_{\alpha\nu} &= -\int_0^\infty dt\,\sum_{mnab}\partial_\alpha h_{nm}(e^{i\underline{\underline{h}}t/\hbar})_{ma}(e^{-i\underline{\underline{h}}t/\hbar})_{bn} tr_e\left(\hat{d}_a^+\hat{d}_b\partial_\nu\hat{\rho}_{ss}\right)\\ &= -\int_0^\infty dt\,\sum_{mnab}\partial_\alpha h_{nm}(e^{i\underline{\underline{h}}t/\hbar})_{ma}\partial_\nu\sigma_{ab}^{ss}(e^{-i\underline{\underline{h}}t/\hbar})_{bn}\\ &= -\int_0^\infty dt\,\mathrm{Tr}_m(\partial_\alpha\underline{\underline{h}}e^{i\underline{\underline{h}}t/\hbar}\partial_\nu\underline{\underline{\sigma}}^{ss}e^{-i\underline{\underline{h}}t/\hbar})\end{aligned} \tag{73}$$

*Electronic Friction At Equilibrium*

At equilibrium, the friction can be further simplified. We transform to the energy domain, just as we did in Eq. 26. Now, the friction reads

$$\begin{aligned}\gamma_{\alpha\nu} &= -\hbar\int\frac{d\epsilon}{2\pi}\mathrm{Tr}_m(\partial_\alpha\underline{\underline{h}}\frac{1}{\epsilon-\underline{\underline{h}}-i\eta}\partial_\nu\underline{\underline{\sigma}}^{ss}\frac{1}{\epsilon-\underline{\underline{h}}+i\eta})\\ &= -\hbar\sum_{kl}\int\frac{d\epsilon}{2\pi}\langle k|\partial_\alpha\underline{\underline{h}}|l\rangle\frac{1}{\epsilon-\epsilon_l-i\eta}\langle l|\partial_\nu\underline{\underline{\sigma}}^{ss}|k\rangle\frac{1}{\epsilon-\epsilon_k+i\eta}\end{aligned} \tag{74}$$

Here, we have expressed the friction in the basis where $\underline{\underline{h}}$ matrix is diagonal

$$\underline{\underline{h}} = \sum_k \epsilon_k |k\rangle\langle k| \tag{75}$$

At equilibrium, we have

$$\underline{\underline{\sigma}}^{ss} = \sum_k f(\epsilon_k)|k\rangle\langle k| \tag{76}$$

We first evaluate

$$\langle l|\partial_\nu \underline{\underline{\sigma}}^{ss}|k\rangle = \partial_\nu \epsilon_k \frac{\partial f(\epsilon_k)}{\partial \epsilon_k}\delta_{kl} + \langle l|\partial_\nu|k\rangle(f(\epsilon_k) - f(\epsilon_l)) \tag{77}$$

Since

$$\partial_\nu \langle l|\underline{\underline{h}}|k\rangle = \partial_\nu \epsilon_k \delta_{lk} = (\epsilon_l - \epsilon_k)\langle l|\partial_\nu|k\rangle + \langle l|\partial_\nu h|k\rangle, \tag{78}$$

this implies that

$$\begin{aligned} \frac{\langle l|\partial_\nu \underline{\underline{h}}|k\rangle}{\epsilon_k - \epsilon_l}(f(\epsilon_k) - f(\epsilon_l)) &= \langle l|\partial_\nu|k\rangle(f(\epsilon_k) - f(\epsilon_l)) + \partial_\nu \epsilon_k \delta_{lk}\frac{f(\epsilon_k) - f(\epsilon_l)}{\epsilon_k - \epsilon_l} \\ &= \langle l|\partial_\nu|k\rangle(f(\epsilon_k) - f(\epsilon_l)) + \partial_\nu \epsilon_k \delta_{lk}\frac{\partial f(\epsilon_k)}{\partial \epsilon_k} \end{aligned} \tag{79}$$

Comparing Eq. 77 and Eq. 79, we have

$$\langle l|\partial_\nu \underline{\underline{\sigma}}^{ss}|k\rangle = \frac{\langle l|\partial_\nu \underline{\underline{h}}|k\rangle}{\epsilon_k - \epsilon_l}(f(\epsilon_k) - f(\epsilon_l)) \tag{80}$$

Using the above results to evaluate the friction, we have

$$\begin{aligned} \gamma_{\alpha\nu} &= -\hbar \int_{-\infty}^{\infty} \frac{d\epsilon}{2\pi} \sum_{kl} \langle k|\partial_\alpha \underline{\underline{h}}|l\rangle \frac{1}{\epsilon - \epsilon_l - i\eta}\langle l|\partial_\nu \underline{\underline{h}}|k\rangle \frac{1}{\epsilon - \epsilon_k + i\eta}\frac{f(\epsilon_k) - f(\epsilon_l)}{\epsilon_k - \epsilon_l} \\ &= -i\hbar \sum_{kl} \langle k|\partial_\alpha \underline{\underline{h}}|l\rangle\langle l|\partial_\nu \underline{\underline{h}}|k\rangle \frac{1}{\epsilon_l - \epsilon_k + 2i\eta}\frac{f(\epsilon_k) - f(\epsilon_l)}{\epsilon_k - \epsilon_l} \end{aligned} \tag{81}$$

At this point, since $\gamma_{\alpha\nu}$ is real and we assume (by ansatz) that $\underline{\underline{h}}$ is real, therefore we can ignore the principal part in the above equation. More generally, if $\underline{\underline{h}}$ were a complex Hermitian, we could also ignore the principal part in the same spirit as the wide band approximation. We then arrive at

$$\begin{aligned} \gamma_{\alpha\nu} &= -\pi\hbar \sum_{kl} \langle k|\partial_\alpha \underline{\underline{h}}|l\rangle\langle l|\partial_\nu \underline{\underline{h}}|k\rangle \delta(\epsilon_l - \epsilon_k)\frac{f(\epsilon_k) - f(\epsilon_l)}{\epsilon_k - \epsilon_l} \\ &= -\pi\hbar \sum_{kl} \int_{-\infty}^{\infty} d\epsilon \, \langle k|\partial_\alpha \underline{\underline{h}}|l\rangle \delta(\epsilon - \epsilon_l)\langle l|\partial_\nu \underline{\underline{h}}|k\rangle \delta(\epsilon_l - \epsilon_k)\frac{\partial f(\epsilon_l)}{\partial \epsilon_l} \\ &= -\pi\hbar \sum_{kl} \int_{-\infty}^{\infty} d\epsilon \, \langle k|\partial_\alpha \underline{\underline{h}}|l\rangle \delta(\epsilon - \epsilon_l)\langle l|\partial_\nu \underline{\underline{h}}|k\rangle \delta(\epsilon - \epsilon_k)\frac{\partial f(\epsilon)}{\partial \epsilon} \\ &= -\pi\hbar \int_{-\infty}^{\infty} d\epsilon \, \mathrm{Tr}_m(\partial_\alpha \underline{\underline{h}}\, \underline{\underline{P}}(\epsilon)\partial_\nu \underline{\underline{h}}\, \underline{\underline{P}}(\epsilon))\frac{\partial f(\epsilon)}{\partial \epsilon} \end{aligned} \tag{82}$$

Here we have defined

$$\underline{\underline{P}}(\epsilon) = \sum_l \delta(\epsilon - \epsilon_l)|l\rangle\langle l| \tag{83}$$

Eqn. 82 agrees with Head-Gordon and Tully [5] at zero temperature and with the conjecture of the results at finite temperature by Tully *et al* in Ref. [7].

As a side-note, we mention that, in the case of a complex $\underline{\underline{h}}$ and without the wide band approximation, the principal part in Eq. 81 would give rise to an asymmetric component of $\gamma_{\alpha\nu}$ along $\alpha$ and $\nu$. Such effects may be interesting and should be investigated further.

### C. Correlation Function of Random Force

The correlation function of the random force by definition is

$$D_{\alpha\nu}(t) = tr_e(\delta\hat{F}_\alpha(t)\delta\hat{F}_\nu(0)\hat{\rho}_{ss}) = \sum_{pqmn} \partial_\alpha h_{qp}\partial_\nu h_{nm} tr_e(e^{i\hat{H}t/\hbar}\hat{d}_p^+\hat{d}_q e^{-i\hat{H}t\hbar}(\hat{d}_m^+\hat{d}_n - \sigma_{mn}^{ss})\hat{\rho}_{ss}) \tag{84}$$

Similar to the previous subsections, we have

$$e^{i\hat{H}t/\hbar}\hat{d}_p^+ e^{-i\hat{H}t/\hbar} = \sum_a (e^{i\underline{\underline{h}}t/\hbar})_{pa}\hat{d}_a^+ \tag{85}$$

$$e^{i\hat{H}t/\hbar}\hat{d}_q e^{-i\hat{H}t/\hbar} = \sum_b (e^{-i\underline{\underline{h}}t/\hbar})_{bq}\hat{d}_b \tag{86}$$

which implies that,

$$D_{\alpha\nu}(t) = \sum_{pqmnab} \partial_\alpha h_{qp}(e^{i\underline{\underline{h}}t/\hbar})_{pa}\partial_\nu h_{nm} tr_e(\hat{d}_a^+\hat{d}_b(\hat{d}_m^+\hat{d}_n - \sigma_{mn}^{ss})\hat{\rho}_{ss})(e^{-i\underline{\underline{h}}t/\hbar})_{bq} \tag{87}$$

For a quadratic Hamiltonian, we can apply Wick's theorem,

$$tr_e(\hat{d}_a^+\hat{d}_b(\hat{d}_m^+\hat{d}_n - \sigma_{mn}^{ss})\hat{\rho}_{ss}) = \sigma_{an}^{ss}(1-\sigma_{mb}^{ss}) \tag{88}$$

The correlation function of random force becomes

$$D_{\alpha\nu}(t) = \sum_{pqmnab} \partial_\alpha h_{qp}(e^{i\underline{\underline{h}}t/\hbar})_{pa}\sigma_{an}^{ss}\partial_\nu h_{nm}(1-\sigma_{mb}^{ss})(e^{-i\underline{\underline{h}}t/\hbar})_{bq} \tag{89}$$

$$= \mathrm{Tr}_m(\partial_\alpha \underline{\underline{h}} e^{i\underline{\underline{h}}t/\hbar}\underline{\underline{\sigma}}^{ss}\partial_\nu \underline{\underline{h}}(1-\underline{\underline{\sigma}}^{ss})e^{-i\underline{\underline{h}}t/\hbar}) \tag{90}$$

We consider fast electronic motion (Markov limit), $D_{\alpha\nu}(t) = 2\bar{D}_{\alpha\nu}\delta(t)$, where

$$\bar{D}_{\alpha\nu} = \int_0^\infty dt\, \mathrm{Tr}_m(\partial_\alpha \underline{\underline{h}} e^{i\underline{\underline{h}}t/\hbar}\underline{\underline{\sigma}}^{ss}\partial_\nu \underline{\underline{h}}(1-\underline{\underline{\sigma}}^{ss})e^{-i\underline{\underline{h}}t/\hbar}) \tag{91}$$

*The Correlation Function of Random Force At Equilibrium*

At equilibrium, $\underline{\underline{\sigma}}^{ss} = f(\underline{\underline{h}})$. In a basis, where $\underline{\underline{h}}$ is diagonal,

$$\begin{aligned}\bar{D}_{\alpha\nu} &= \hbar\int \frac{d\epsilon}{2\pi}\sum_{kl}\langle k|\partial_\alpha \underline{\underline{h}}|l\rangle \frac{1}{\epsilon-\epsilon_l-i\eta}(1-f(\epsilon_l))\langle l|\partial_\nu \underline{\underline{h}}|k\rangle\frac{1}{\epsilon-\epsilon_k+i\eta}f(\epsilon_k)\\ &= i\hbar\sum_{kl}\langle k|\partial_\alpha \underline{\underline{h}}|l\rangle(1-f(\epsilon_l))\langle l|\partial_\nu \underline{\underline{h}}|k\rangle\frac{1}{\epsilon_l-\epsilon_k+2i\eta}f(\epsilon_k)\end{aligned} \tag{92}$$

Since, $\bar{D}_{\alpha\nu}^S = \mathrm{Re}(\bar{D}_{\alpha\nu})$, if $\underline{\underline{h}}$ is real or if $\underline{\underline{h}}$ is complex (but the wide band approximation applies), we can ignore the principal part of Eq. 92, and so

$$\begin{aligned}\bar{D}_{\alpha\nu}^S &= \pi\hbar\sum_{kl}\langle k|\partial_\alpha \underline{\underline{h}}|l\rangle(1-f(\epsilon_l))\langle l|\partial_\nu \underline{\underline{h}}|k\rangle\delta(\epsilon_l-\epsilon_k)f(\epsilon_k)\\ &= \pi\hbar\sum_{kl}\int d\epsilon\langle k|\partial_\alpha \underline{\underline{h}}|l\rangle\delta(\epsilon-\epsilon_l)\langle l|\partial_\nu \underline{\underline{h}}|k\rangle\delta(\epsilon_l-\epsilon_k)f(\epsilon_k)(1-f(\epsilon_l))\\ &= \pi\hbar\sum_{kl}\int d\epsilon\langle k|\partial_\alpha \underline{\underline{h}}|l\rangle\delta(\epsilon-\epsilon_l)\langle l|\partial_\nu \underline{\underline{h}}|k\rangle\delta(\epsilon-\epsilon_k)f(\epsilon)(1-f(\epsilon))\\ &= \pi\hbar\int d\epsilon\, \mathrm{Tr}_m(\partial_\alpha \underline{\underline{h}}\,\underline{\underline{P}}(\epsilon)\partial_\nu \underline{\underline{h}}\,\underline{\underline{P}}(\epsilon))f(\epsilon)(1-f(\epsilon))\end{aligned} \tag{93}$$

As we mentioned above, in the case of a complex $\underline{\underline{h}}$ without the wide band approximation, the principal part in Eq. 92 give rise to an asymmetric component of $\bar{D}_{\alpha\nu}^S$ along $\alpha$ and $\nu$. Such effects should be investigated in the future.

Eq. 93 was not derived by Head-Gordon and Tully, but does satisfy the second fluctuation-dissipation theorem with Eq. 82. Furthermore, in a future article, we will show that Eqs. 93 and 82 are also in complete agreement with von Oppen *et al* [6].

## VI. AN EFFECTIVE LIOUVILLIAN APPROACH: FRICTION AND MASTER EQUATIONS

Before concluding, let us connect the present universal picture of electronic friction (Eq. 23) with another expression for friction published previously [1]. In Ref. [1], we considered a special Hamiltonian, whereby we could divide all of the world's electronic DoF's into system and bath electrons. The dynamics of the system electronic DoFs, which were coupled with nuclear DoF's, followed an effective Liouvillian $\hat{\hat{\mathcal{L}}}_{eff}$ as obtained by a quantum master equation:

$$\dot{\hat{\rho}}_{sys} = -\hat{\hat{\mathcal{L}}}_{eff}\hat{\rho}_{sys} \tag{94}$$

The effective Liouvillian for the system contains explicit dissipation due to coupling to the bath. Following the same derivation in Sec. I of this SM, we now find the following expression for friction

$$\gamma^{eff}_{\alpha\nu} = -tr_{sys}\Big(\partial_\alpha \hat{H}_{sys}\hat{\hat{\mathcal{L}}}^{-1}_{eff}\partial_\nu \hat{\rho}^{ss}_{sys}\Big) \tag{95}$$

while the correlation function for the random force is

$$\bar{D}^{eff}_{\alpha\nu} = \frac{1}{2}tr_{sys}\left(\partial_\alpha \hat{H}_{sys}\hat{\hat{\mathcal{L}}}^{-1}_{eff}\Big(\partial_\nu \hat{H}_{sys}\hat{\rho}^{ss}_{sys} + \hat{\rho}^{ss}_{sys}\partial_\nu \hat{H}_{sys} - 2tr_{sys}(\hat{\rho}^{ss}_{sys}\partial_\nu \hat{H}_{sys})\hat{\rho}^{ss}_{sys}\Big)\right) \tag{96}$$

Here $tr_{sys}$ implies tracing over system electronic DoF's, and $\hat{\rho}^{ss}_{sys}$ is the system steady state density matrix. Eqs. 95-96 were derived previously in Ref. [1]. Because the effective Liouvillian was derived from a quantum master equation, Eqs. 95-96 do not properly treat level broadening effects [1]. Furthermore, because a quantum master expression introduces explicit relaxation and breaks time-reversibility, neither the friction nor the correlation function for the random force in Eqs. 95 - 96 is guaranteed to be symmetric along $\alpha$ and $\nu$.

## VII. NON-MARKOVIAN FOKKER-PLANCK EQUATION

In this final section of the SM, we will now extend the Fokker-Planck equation from Sec. I B to the non-Markovian limit (which will connect with Ref. [8]) and introduce the simplest possible form of memory. Following Sec. I B, we start from the EOM for $\mathcal{A}$ and $\hat{\mathcal{B}}$

$$\partial_t \mathcal{A} = -\sum_\alpha \frac{P_\alpha}{m_\alpha}\partial_\alpha \mathcal{A} + \sum_\alpha tr_e(\partial_\alpha \hat{H}\hat{\rho}_{ss})\frac{\partial \mathcal{A}}{\partial P_\alpha} + \sum_\alpha tr_e(\partial_\alpha \hat{H}\frac{\partial \hat{\mathcal{B}}}{\partial P_\alpha}) \tag{97}$$

$$\partial_t \hat{\mathcal{B}} = \{\hat{H}_{tot}, \hat{\mathcal{B}}\}_a - \hat{\rho}_{ss}tr_e\{\hat{H}_{tot}, \hat{\mathcal{B}}\}_a + \{\hat{H}_{tot}, \mathcal{A}\hat{\rho}_{ss}\}_a - \hat{\rho}_{ss}tr_e\{\hat{H}_{tot}, \mathcal{A}\hat{\rho}_{ss}\}_a - \hat{\hat{\mathcal{L}}}\hat{\mathcal{B}} \tag{98}$$

At this point, we make a slightly different approximation so that we replace Eq. 39 by the following:

$$\partial_t \hat{\mathcal{B}} = \{\hat{H}_{tot}, \mathcal{A}\hat{\rho}_{ss}\}_a - \hat{\rho}_{ss}tr_e\{\hat{H}_{tot}, \mathcal{A}\hat{\rho}_{ss}\}_a - \hat{\hat{\mathcal{L}}}\hat{\mathcal{B}} \tag{99}$$

We now solve for $\hat{\mathcal{B}}$

$$\hat{\mathcal{B}}(t) = e^{-\hat{\hat{\mathcal{L}}}t}\hat{\mathcal{B}}(0) + \int_0^t dt' e^{-\hat{\hat{\mathcal{L}}}(t-t')}\Big(\{\hat{H}_{tot}, \mathcal{A}(t')\hat{\rho}_{ss}\}_a - \hat{\rho}_{ss}tr_e\{\hat{H}_{tot}, \mathcal{A}(t')\hat{\rho}_{ss}\}_a\Big) \tag{100}$$

We assume that, at $t = 0$, the total system is at equilibrium, i.e. $\hat{\mathcal{B}}(0) = 0$. Then, if we plug the above equation into the EOM for $\mathcal{A}$ (Eq. 97), we arrive at a non-Markovian Fokker-Planck equation,

$$\partial_t \mathcal{A}(t) = -\sum_\alpha \frac{P_\alpha}{m_\alpha}\partial_\alpha \mathcal{A}(t) - \sum_\alpha F_\alpha \frac{\partial \mathcal{A}(t)}{\partial P_\alpha} + \sum_{\alpha\nu}\int_0^t dt' \tilde{\gamma}_{\alpha\nu}(t-t')\frac{\partial}{\partial P_\alpha}(\frac{P_\nu}{m_\nu}\mathcal{A}(t')) + \sum_{\alpha\nu}\int_0^t dt' D^S_{\alpha\nu}(t-t')\frac{\partial^2 \mathcal{A}(t')}{\partial P_\alpha \partial P_\nu} \tag{101}$$

where

$$\tilde{\gamma}_{\alpha\nu}(t-t') = -tr_e\Big(\partial_\alpha \hat{H} e^{-\hat{\hat{\mathcal{L}}}(t-t')}\partial_\nu \hat{\rho}_{ss}\Big) \tag{102}$$

$$D^S_{\alpha\nu}(t-t') = \frac{1}{2}tr_e\Big(\delta\hat{F}_\alpha e^{-\hat{\hat{\mathcal{L}}}(t-t')}\big(\delta\hat{F}_\nu \hat{\rho}_{ss} + \hat{\rho}_{ss}\delta\hat{F}_\nu\big)\Big) \tag{103}$$

It is easy to verify that, in the Makovian limit, the above equation (Eq. 101) reduces to the Fokker-Planck equation in Sec. I B (Eq. 40).

Let us now show that the second fluctuation-dissipation theorem still holds at equilibrium (at least approximately). At equilibrium, $\hat{\rho}_{ss} = e^{-\hat{H}/k_BT}/Z$, where $Z = tr_e(e^{-\hat{H}/k_BT})$, so that the following relationship holds in the semi-classical limit [9],

$$\partial_\nu e^{-\hat{H}/k_BT} = -\frac{1}{2k_BT}(\partial_\nu \hat{H} e^{-\hat{H}/k_BT} + e^{-\hat{H}/k_BT}\partial_\nu \hat{H}) \tag{104}$$

Thus,

$$\partial_\nu \hat{\rho}_{ss} = -\frac{1}{2k_BT}\Big(\partial_\nu \hat{H}\hat{\rho}_{ss} + \hat{\rho}_{ss}\partial_\nu \hat{H} - 2tr_e(\partial_\nu \hat{H}\hat{\rho}_{ss})\hat{\rho}_{ss}\Big) = \frac{1}{2k_BT}(\delta\hat{F}_\nu \hat{\rho}_{ss} + \hat{\rho}_{ss}\delta\hat{F}_\nu) \tag{105}$$

and the second fluctuation-dissipation theorem can be verified:

$$\tilde{\gamma}_{\alpha\nu}(t) = \frac{1}{2k_BT}tr_e\Big(\delta\hat{F}_\alpha(t)\big(\delta\hat{F}_\nu\hat{\rho}_{ss} + \hat{\rho}_{ss}\delta\hat{F}_\nu\big)\Big) = \frac{1}{k_BT}D^S_{\alpha\nu}(t) \tag{106}$$

Here we have defined

$$\delta\hat{F}_\alpha(t) = e^{i\hat{H}t}\delta\hat{F}_\alpha e^{-i\hat{H}t} \tag{107}$$

To further connect our results to those in Ref. [8], we can perform a Laplace transform, which is defined as

$$\delta\hat{F}_\alpha(s) = \int_0^\infty dt\, \delta\hat{F}_\alpha(t)e^{-st} \tag{108}$$

After a Laplace transform, the friction reads

$$\tilde{\gamma}_{\alpha\nu}(s) = \frac{1}{2k_BT}tr_e\Big(\delta\hat{F}_\alpha(s)\big(\delta\hat{F}_\nu\hat{\rho}_{ss} + \hat{\rho}_{ss}\delta\hat{F}_\nu\big)\Big) \tag{109}$$

Eq. 109 agrees with Eq. 3.18 in Ref. [8]. Note, however, that the Ref. [8] worked with a one-dimensional nuclear coordinate. For a mulitdimensional system, one must symmetrize the force-force correlation function, as in Eq. 109.

[1] W. Dou and J. E. Subotnik, J. Chem. Phys. **145**, 054102 (2016).
[2] R. Kapral and G. Ciccotti, J. Chem. Phys. **110**, 8919 (1999).
[3] R. Bulla, T. A. Costi, and T. Pruschke, Rev. Mod. Phys. **80**, 395 (2008).
[4] A. A. Dzhioev, D. S. Kosov, and F. von Oppen, J. Chem. Phys. **138**, 134103 (2013).
[5] M. Head-Gordon and J. C. Tully, J. Chem. Phys. **103**, 10137 (1995).
[6] N. Bode, S. V. Kusminskiy, R. Egger, and F. von Oppen, Beilstein J. Nanotechnol **3**, 144 (2012).
[7] R. J. Maurer, M. Askerka, V. S. Batista, and J. C. Tully, Phys. Rev. B **94**, 115432 (2016).
[8] B. B. Smith and J. T. Hynes, J. Chem. Phys. **99**, 6517 (1993).
[9] R. Kapral, Ann. Rev. Phys. Chem. **57**, 129 (2006).
